# Supplementary material for: Astra: Toward General-Purpose Mobile Robots via Hierarchical Multimodal Learning
Source: arXiv:2506.06205 source file (2025-06-06)
Supplement: Supplementary file 1 [file appendix.tex]

\section{Appendix}
\label{appendix}

Other similar interactions with forklift in a warehouse and with person in a building are shown in Fig.~\ref{fig:case-dynamic2}, \ref{fig:case-dynamic3}, where the model enables safer obstacle avoidance behaviors against the moving objects.

\begin{figure}[ht]
    \centering
    \begin{subfigure}{\textwidth}
        \includegraphics[width=\textwidth, height=\imgcaseheight]{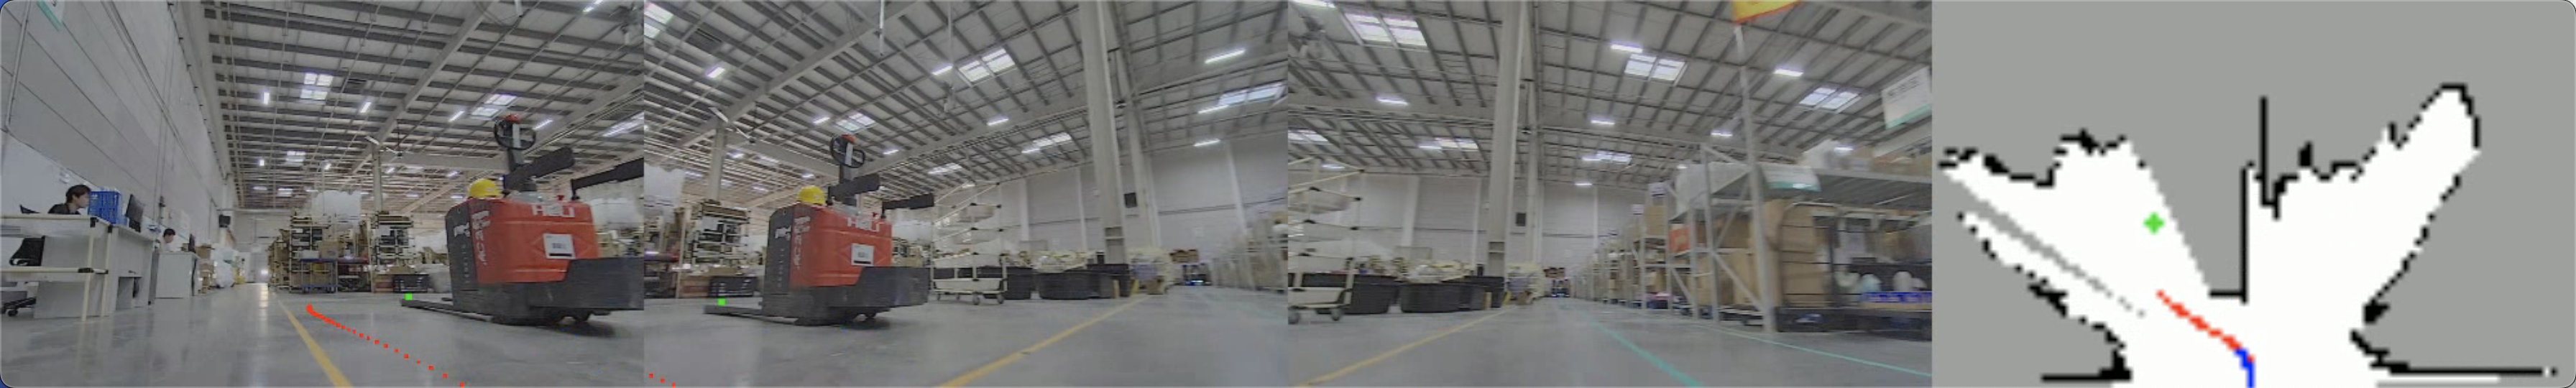} 
    \end{subfigure}
    
    \begin{subfigure}{\textwidth}
        \includegraphics[width=\textwidth, height=\imgcaseheight]{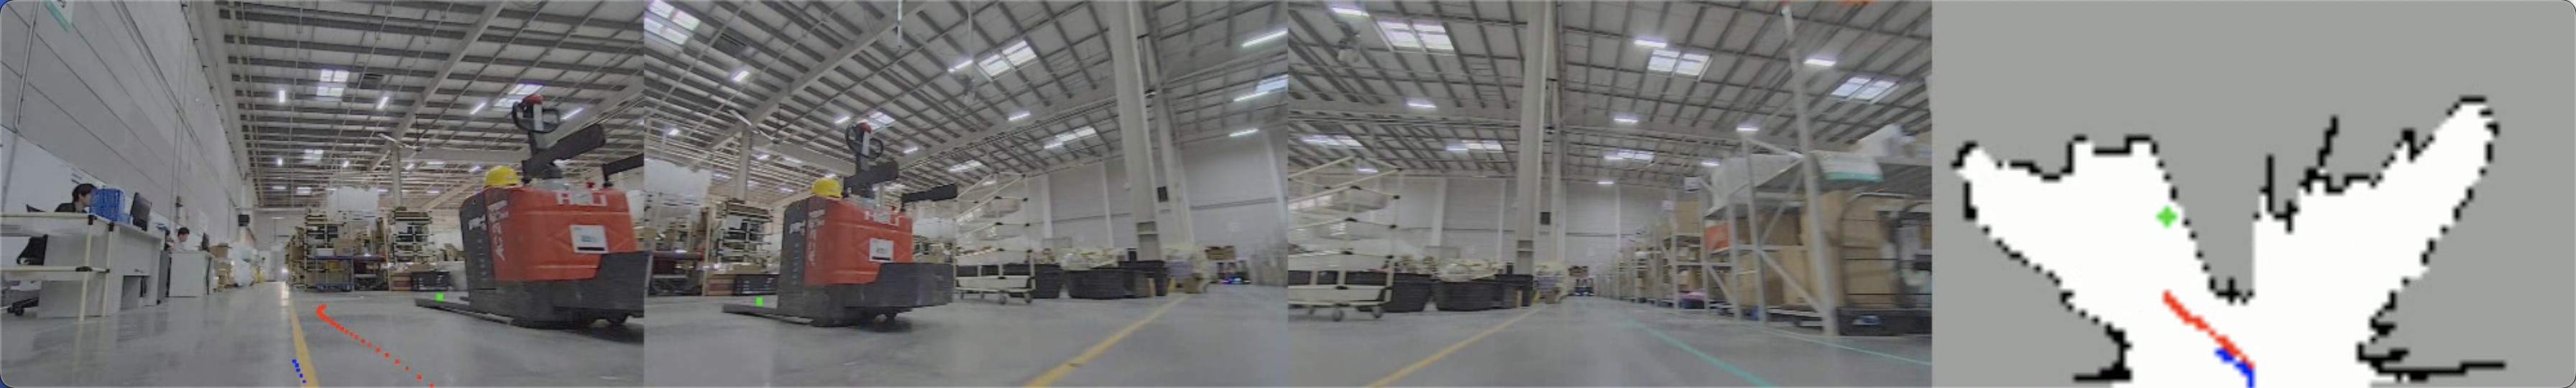}
    \end{subfigure}
    
    \begin{subfigure}{\textwidth}
        \includegraphics[width=\textwidth, height=\imgcaseheight]{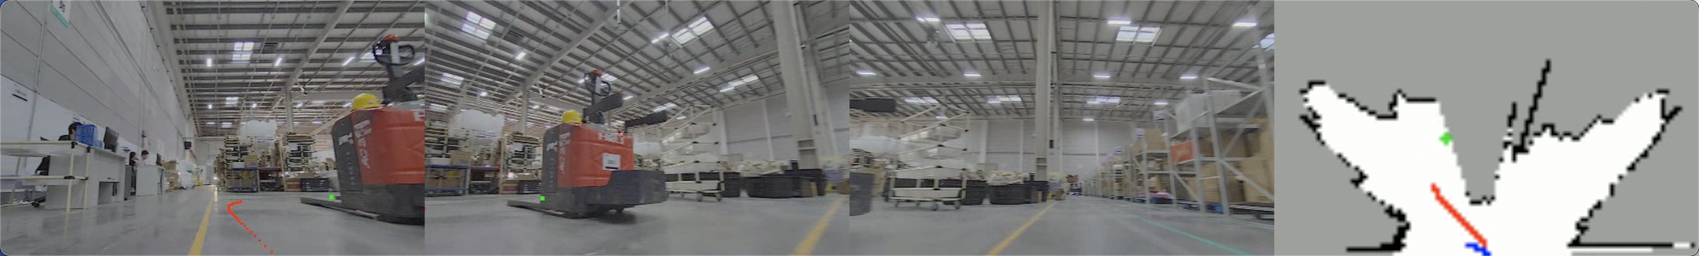}
    \end{subfigure}
    
    \begin{subfigure}{\textwidth}
        \includegraphics[width=\textwidth, height=\imgcaseheight]{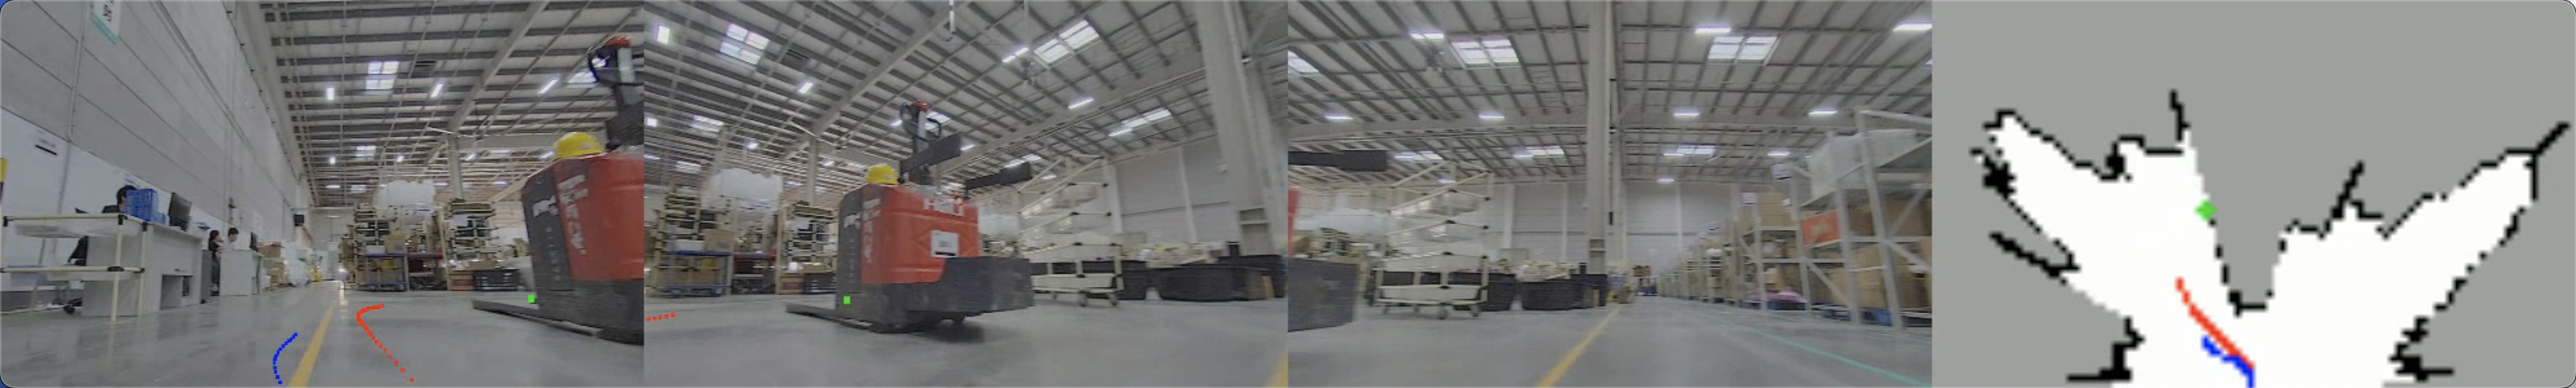}
    \end{subfigure}
    \caption{Case study: interaction with a forklift in a warehouse.}
    \label{fig:case-dynamic2}
\end{figure}

\begin{figure}[ht]
    \centering
    \begin{subfigure}{\textwidth}
        \includegraphics[width=\textwidth, height=\imgcaseheight]{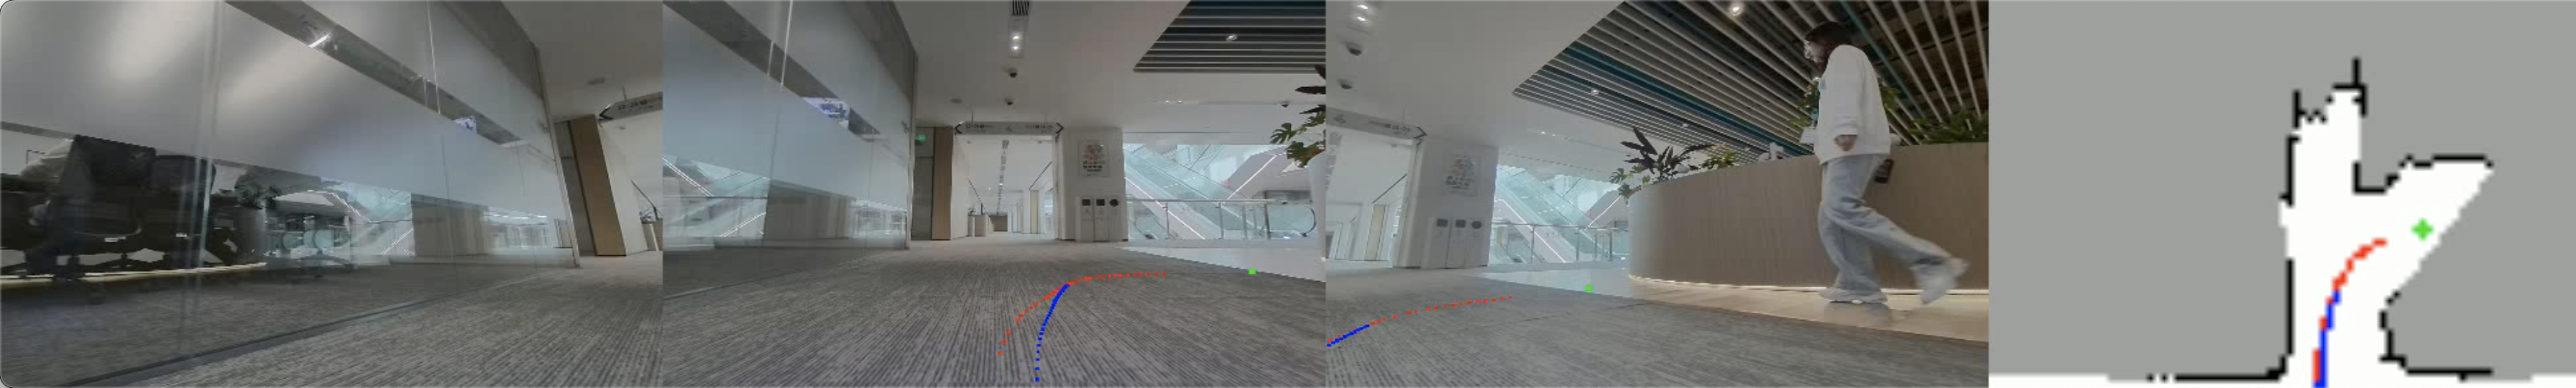} 
    \end{subfigure}
    
    \begin{subfigure}{\textwidth}
        \includegraphics[width=\textwidth, height=\imgcaseheight]{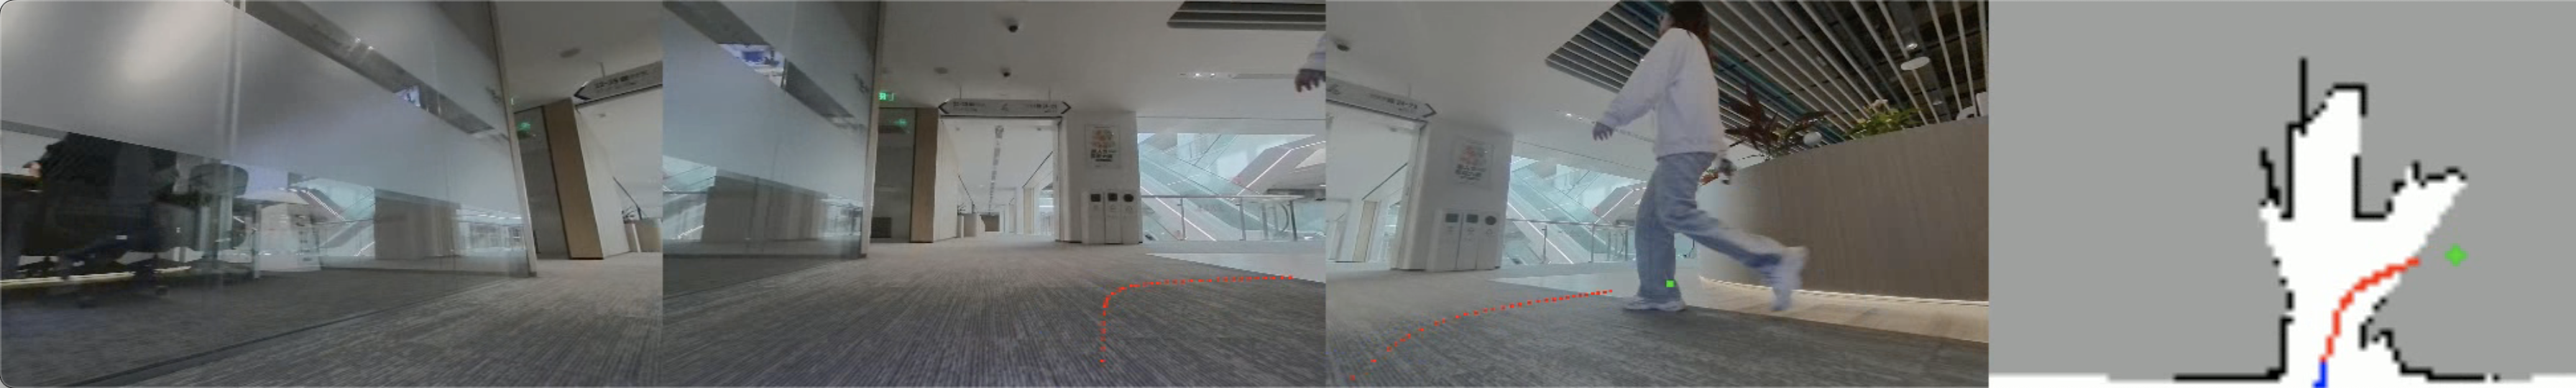}
    \end{subfigure}
    
    \begin{subfigure}{\textwidth}
        \includegraphics[width=\textwidth, height=\imgcaseheight]{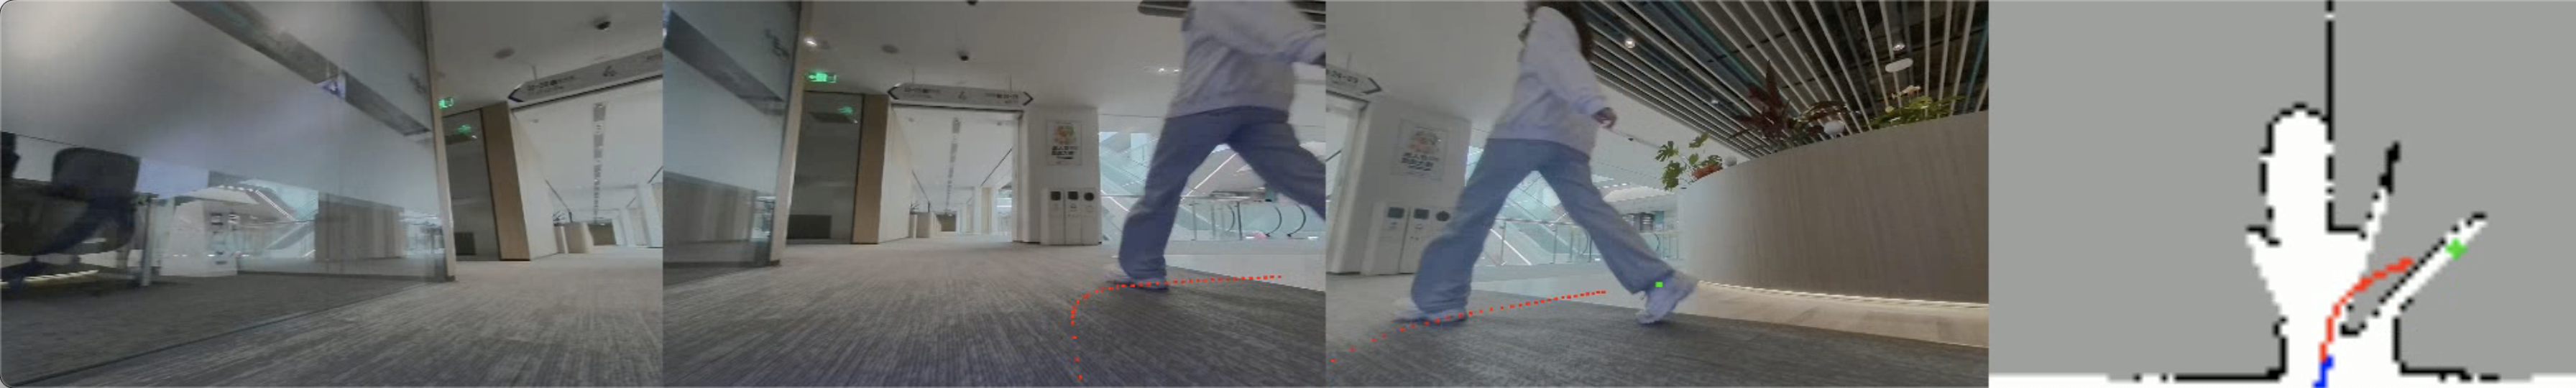}
    \end{subfigure}
    
    \begin{subfigure}{\textwidth}
        \includegraphics[width=\textwidth, height=\imgcaseheight]{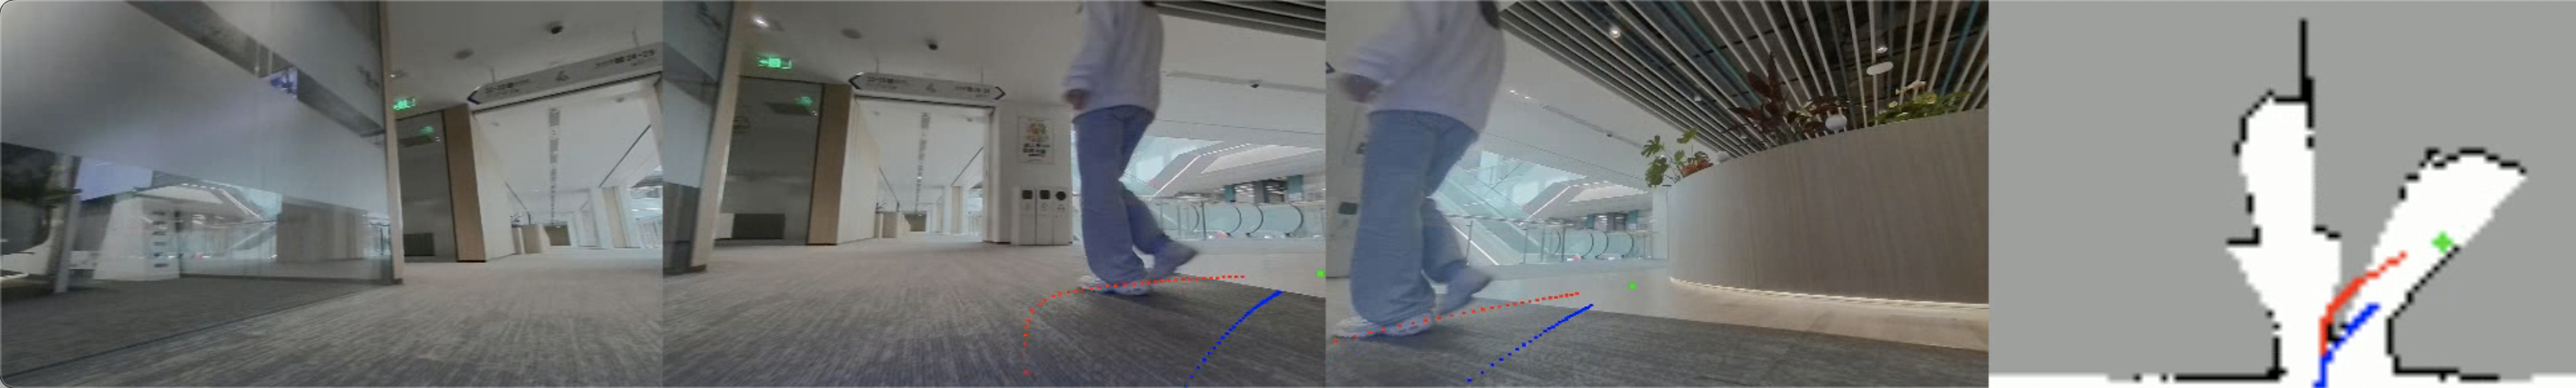}
    \end{subfigure}
    \caption{Case study: interaction with a person in a building.}
    \label{fig:case-dynamic3}
\end{figure}
